# Supplementary material for: Deep Ensembles Work, But Are They Necessary?
Source: arXiv:2202.06985 source file (2022-10-13)
Supplement: Supplementary file 1 [file other_decomposition.tex]

\section{Negative Log Likelihood decomposition into epistemic and aleatoric uncertainty}

We can follow the same rationale for the negative log likelihood as we did for the Brier score in order to relate the ensemble and average single model negative log likelihoods. For a given data point ${x,y}$ as above, we have $p^*_i(x)$ as the likelihood of the true class, given by model $i$, $i\in {1\dots M}$. We can then write: 

\begin{align*}
    -\log\left(\frac{1}{M}\sum_i p_i^*\right) -\frac{1}{M}\sum -\log (p_i^*) &= - \frac{1}{M} \sum \left[ -\log p_i^* +\log\left(\frac{1}{M}\sum p_i^*\right)\right] \\
    &= -\frac{1}{M}\sum \log \left( \frac{\frac{1}{M}}{\frac{p^*_i}{\sum p^*_i}} \right) \\ 
    &= -\sum \frac{1}{M}\log\left(\frac{\frac{1}{M}}{\frac{p^*_i}{\sum p^*_i}}\right) \\
    &= -D_{KL}(P\|Q)
\end{align*}
In this expression, $P$ is the uniform distribution over $M$ classes and $Q$ is the distribution of normalized likelihoods from all ensemble members, $\frac{p^*_i}{\sum p^*_i}$.
This final term measures ensemble diversity as the Kullback-Liebler divergence between the maximum entropy distribution on the set of $M$ elements, and the distribution of likelihoods output by ensemble members. 

\section{Relating Linear Trends to Ensemble Diversity \label{sec:lindiv}}
Assume that we have constants $c_0, c_1$ such that we have $\E_{p_{ood}(\vx, y)}[B_{ood}(f_i)] = c_0*\E_{p_{ind}(\vx, y)}[B_{ind}(f_i)]+c_1$. Then, we can write the ensemble Brier Score as: 
\begin{align}
   &\E_{p_{ood}(\vx, y)}[B_{ood}(\bar \vf)] = c_0*\E_{p(\vx_{ind}, y)}[B_{ind}(\bar \vf)]+c_1 \\
  \implies &E_{p_{ood}(\vx, y)}[\E_\vf \left[ B_{ood}(\vf) \right]
    - \Var_{ood}\|\vf(x)\|_2] = \\
 &c_0* [ \E_{p_{ind}(\vx, y)}[B_{ind}(\vf)
    - \Var_{ind}\|\vf(x)\|_2] ] +c_1 \\
\implies &\frac{\E_{p_{ood}(\vx, y)}[\Var_{ood}\|\vf(x)\|_2]]}{\E_{p_{ind}(\vx, y)}[\Var_{ind}\|\vf(x)\|_2]} = c_0 \tag{Average model is also collinear}     \\ 
\implies &\frac{\E_{\vf(x_{ind})}[\E[\Var_{ood}\|\vf(x)\|_2\mid \E_{\vf}[1-\|\vf(x)\|]  ]]}{\E_{\vf(x_{ood})}[\E [\Var_{ind}\|\vf(x)\|_2\mid \E_{\vf}[1-\|\vf(x)\|]]]} = c_0 \tag{Law of unconscious statistician, tower property of expectation} 
\end{align}

\section{Decomposition for proper scores.}
\label{sec:decomposition_prop_scores}

To better understand the contribution of ensemble diversity to these linear trends, we can apply bias-variance decompositions to these proper scoring rules just as we applied them to the total uncertainty in section \ref{sec:metricepiun}.
In particular, the ensemble Brier Score yields the following decomposition: 

\begin{align*}
    \E_{p(\vx, y)}[ B_p(\bar \vf) ]&= \E_{p(\vx, y)}[\E_\vf \left[ B_p(\vf) \right]
    - \Var\|\vf(x)\|_2]
\end{align*}

the ensemble NLL likewise yields the decomposition: 

\begin{align*}
    \E_{p(\vx, y)}[&-\log\left(\frac{1}{M}\sum_i p_i^*\right)] \\ &=  \E_{p(\vx, y)}[\frac{1}{M}\sum -\log (p_i^*)
     -D_{KL}(P\|Q)]
\end{align*}

Here $P$ is the uniform distribution over a set of $M$ elements and $Q$ is the normalized distribution of likelihoods, $\frac{p_i^8}{\sum p_i^*}$. See appendix B,C,D for details. 

Given the collinearity of ensembles and single models, we can analyze the role of ensemble diversity alone for these metrics. Assume that we have constants $c_0, c_1$ such that we have $\E_{p_{ood}(\vx, y)}[B_{ood}(f_i)] = c_0*\E_{p_{ind}(\vx, y)}[B_{ind}(f_i)]+c_1$. Then, for the ensemble Brier Score: 
\begin{align}
   &\E_{p_{ood}(\vx, y)}[B_{ood}(\bar \vf)] = c_0*\E_{p(\vx_{ind}, y)}[B_{ind}(\bar \vf)]+c_1 \\
\implies &\frac{\E_{\vf(x_{ind})}[\E[\Var_{ood}\|\vf(x)\|_2\mid \E_{\vf}[1-\|\vf(x)\|]  ]]}{\E_{\vf(x_{ood})}[\E [\Var_{ind}\|\vf(x)\|_2\mid \E_{\vf}[1-\|\vf(x)\|]]]} = c_0  
\end{align}

See Appendix D for derivation. This equation tells us that the relationship between the in and out of distribution variance of these ensembles is tightly determined given that ensembles are collinear with single models. 
The quantity $\E[\Var\|\vf(x)\|_2\mid \E_{\vf}[1-\|\vf(x)\|]]$ is exactly what we plot in Figure \ref{fig:f0}. We can see from this derivation that a sufficient condition to simultaneously 1) improve the quality of ensemble diversity as a measure of epistemic uncertainty and 2) to increase the robustness of ensembles relative to single models would be to increase $\E[\Var_{ood}\|\vf(x)\|_2\mid \E_{\vf}[1-\|\vf(x)\|]]$ relative to $\E[\Var_{ind}\|\vf(x)\|_2\mid \E_{\vf}[1-\|\vf(x)\|]]$. 
Similar derivations can be made for the Negative Log Likelihood \ta{derive/plot these}.
