# Supplementary material for: Deep Ensembles Work, But Are They Necessary?
Source: arXiv:2202.06985 source file (2022-10-13)
Supplement: Supplementary file 2 [file scratch.tex]

\section{Scratch}
Why do we see that the pattern of ensemble generalization is so well determined by single model generalization?
We’d like to be able to understand this phenomenon at the level of the data distribution next.

\paragraph{Notation.} \gp{Move this paragraph somewhere else.}
Let $\vx \in \R^D$ be an input and $y \in [1, C]$ be its target, where $D$ is the number of features and $C$ is the number of classes.
A single model $\vf : \R^D \to \Delta^C$ maps an input to the $C$-class probability simplex.
Given a set of models $\vf_1, \ldots, \vf_M$,
let $\bar \vf(\vx) = 1/M \sum_{i=1}^M \vf_i(\vx)$ represent the ensemble of models.
We will also represent ensemble members as a discrete distribution over possible models:
$p(\vf) = \text{Unif.} [ \vf_1, \ldots, \vf_M ] $.

One reasonable definition for the total uncertainty of an ensemble is $U(\vx) = 1 - \Vert \bar\vf(\vx) \Vert_2^2$.
$U(\vx)$ will be small when all ensemble members agree and express high confidence in a single class.
Conversely, $U(\vx)$ will be large when ensemble members disagree, or when ensemble members express low confidence in all classes.
Furthermore, $U(\vx)$ can be decomposed into interpretable terms:
\begin{align}
    U(\vx) &\triangleq 1 - \Vert \bar\vf(\vx) \Vert_2^2
    \nonumber \\
    &= \underbracket{
        \left( \E_{\vf} \left[ \Vert \vf(\vx) \Vert_2^2 \right] - \Vert \bar\vf(\vx) \Vert_2^2 \right)
    }_{\Var[ \Vert \vf(\vx) \Vert_2 ]}
    \label{eqn:sq_epistemic1}
    \\
    &\phantom{=} + \E_{\vf} \left[ \left( 1 - \Vert \vf(\vx) \Vert_2^2 \right) \right]
    \label{eqn:sq_aleatoric1}
\end{align}
Note that \cref{eqn:sq_aleatoric} measures disagreement between ensembles,
and thus can be interpreted as a notion of epistemic uncertainty.
Conversely, \cref{eqn:sq_epistemic} captures the average aleatoric uncertainty expressed by ensemble members.

Consider the average Brier score across individual models:
\begin{align}
    \E_\vf \left[ B_p(\vf) \right] &= \E_{p(\vx, y)} \E_\vf \left[ \Vert \vf(\vx) - \vone_y \Vert_2^2 \right]
    \label{eqn:avg_brier} \\
    &= \E_{p(\vx, y)} \left[
        \E_\vf \left[ \Vert \vf(\vx) \Vert_2^2 \right]
        + 2 \bar \vf(\vx)^\top \vone_y
        + 1
    \right]
    \nonumber
\end{align}
and the Brier score of the ensemble:
\begin{align}
    B_p(\bar \vf) &= \E_{p(\vx, y)} \left[ \Vert \bar \vf(\vx) - \vone_y \Vert_2^2 \right]
    \label{eqn:ens_brier} \\
    &= \E_{p(\vx, y)} \left[
        \Vert \bar \vf(\vx) \Vert_2^2
        + 2 \bar \vf(\vx)^\top \vone_y
        + 1
    \right]
    \nonumber
\end{align}
Note that \cref{eqn:avg_brier} and \cref{eqn:ens_brier} only differ by a single term:
\begin{align*}
    B_p(\bar \vf) &= \E_\vf \left[ B_p(\vf) \right]
    + \E_{p(\vx)} \left[ \Vert \bar \vf(\vx) \Vert_2^2  \right]
    \\ &\phantom{=}
    - \E_{p(\vx)} \E_\vf \left[ \Vert \vf(\vx) \Vert_2^2 \right].
\end{align*}

Now assume that we see a linear relationship between InD and OOD Brier score for individual models:
\[
    B_q(\bar \vf) = c_0 B_p(\bar \vf) + c_1
\]
where $p(\vx, y)$ and $q(\vx, y)$ represent the InD and OOD data distributions, respectively,
and $c_0$ and $c_1$ represent some constants.
Consequentially, the OOD Brier score can be written as a linear combination of the InD terms in \cref{eqn:avg_brier}.
\begin{align*}
    B_q(\bar \vf)
    = c'_0 \E_{p(\vx)} \left[
        \E_\vf \left[ \Vert \vf(\vx) \Vert_2^2 \right]
    \right]
    \\
    + c'_1 \E_{p(\vx, y)} \left[
        \bar \vf(\vx)^\top \vone_y
    \right]
    + c'_2,
\end{align*}
where $c'_0 = $
